# Supplementary material for: Maximum Likelihood de novo reconstruction of viral populations using paired end sequencing data
Source: arXiv:1502.04239 source file (2016-04-16)
Supplement: Supplementary file 1 [file SupplementaryFile.pdf]

S1 Figure

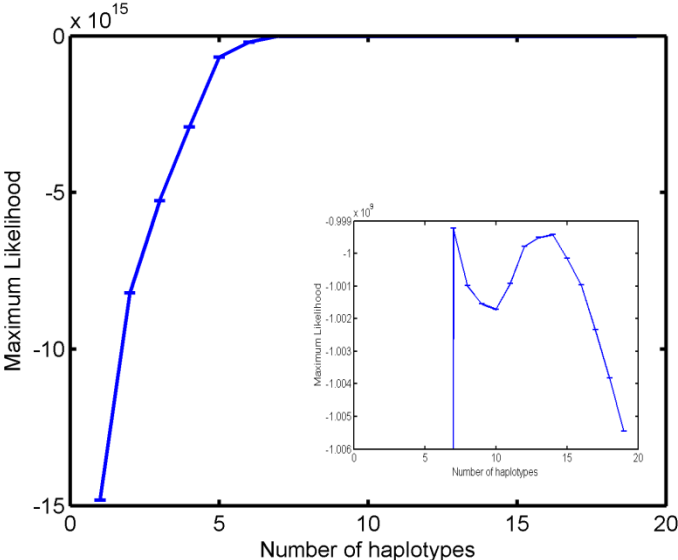

D1

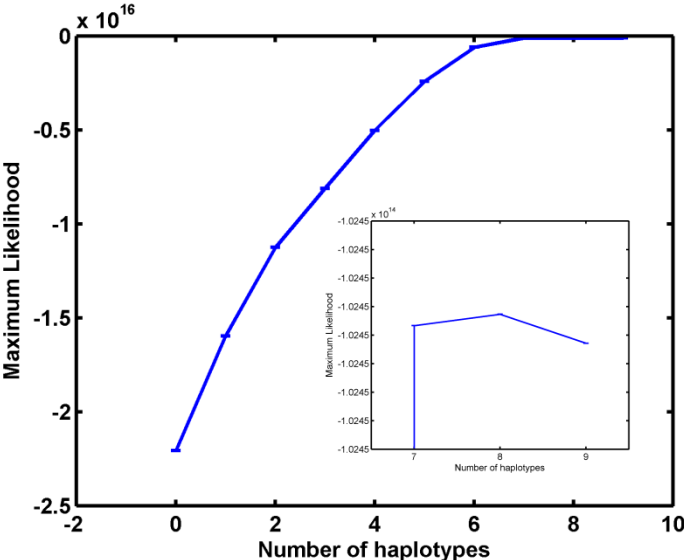

D8

## S2 Figure

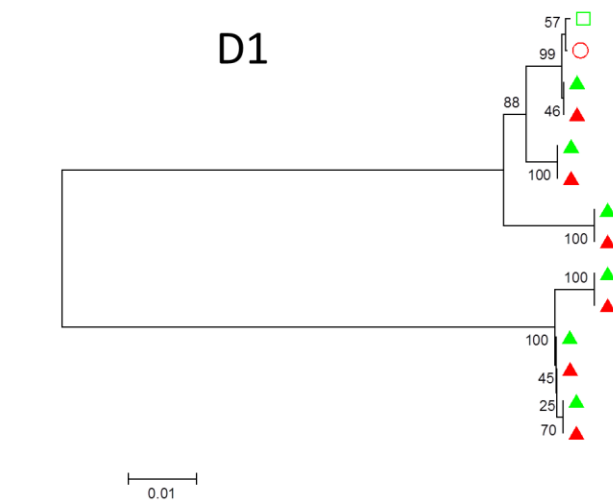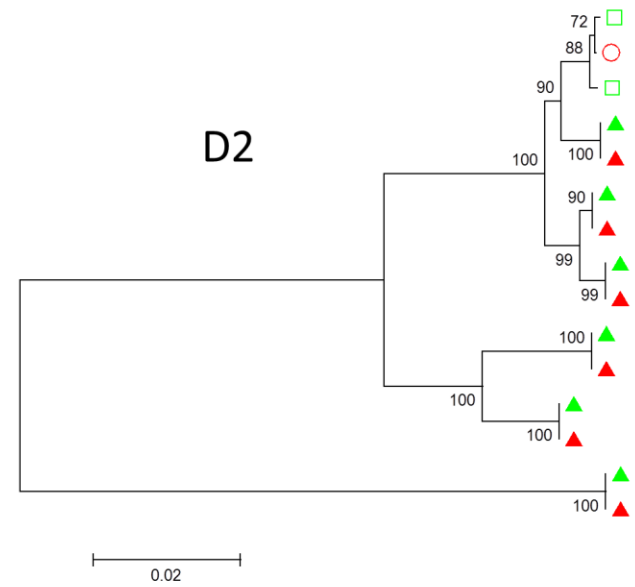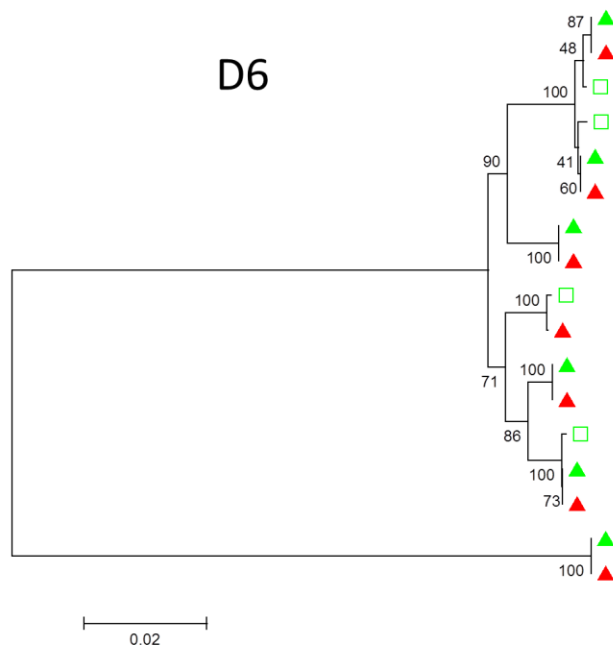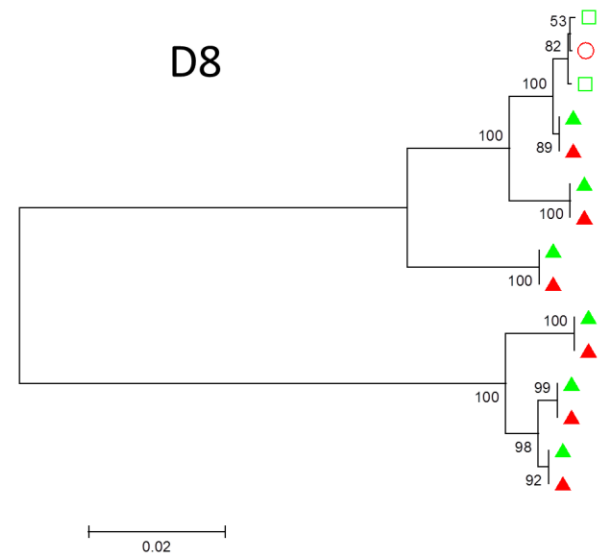

## S3 Figure

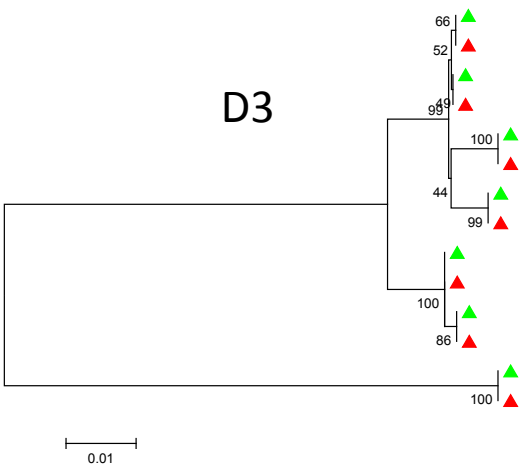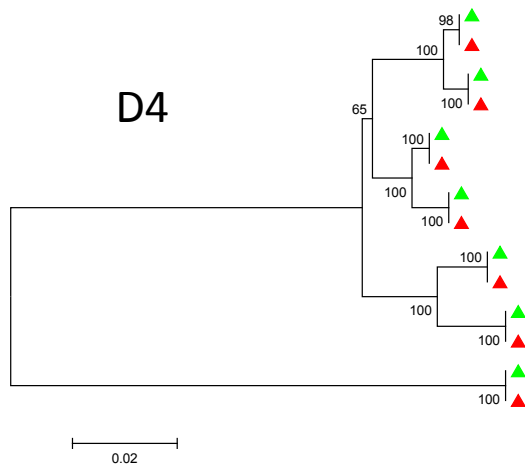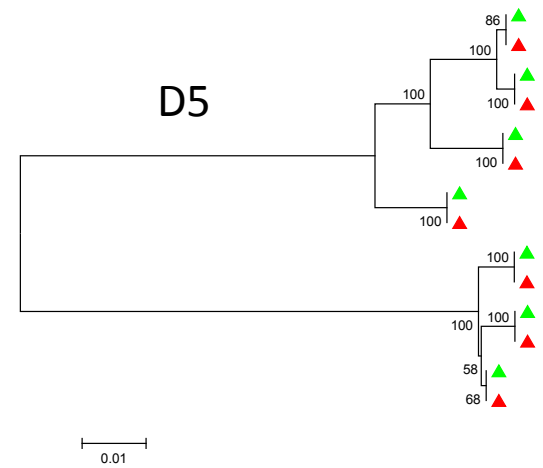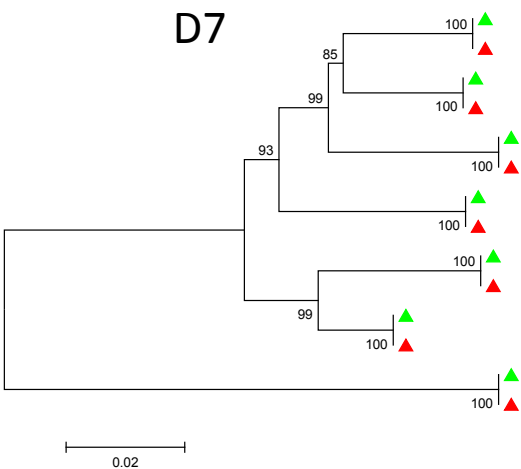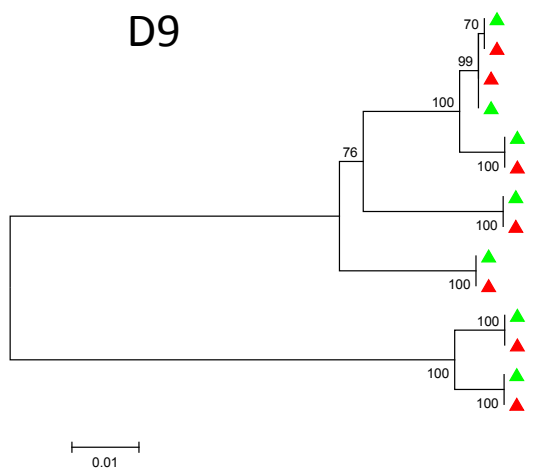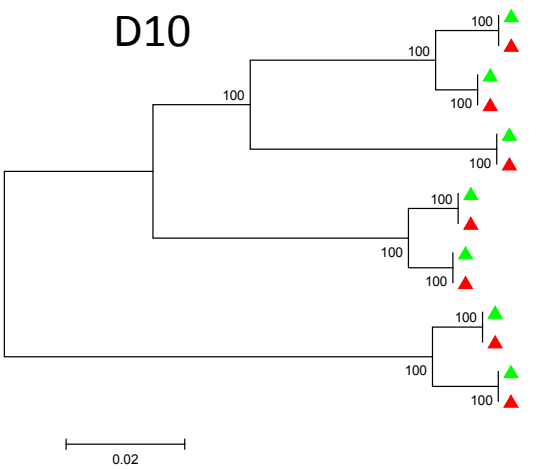

S4 Figure

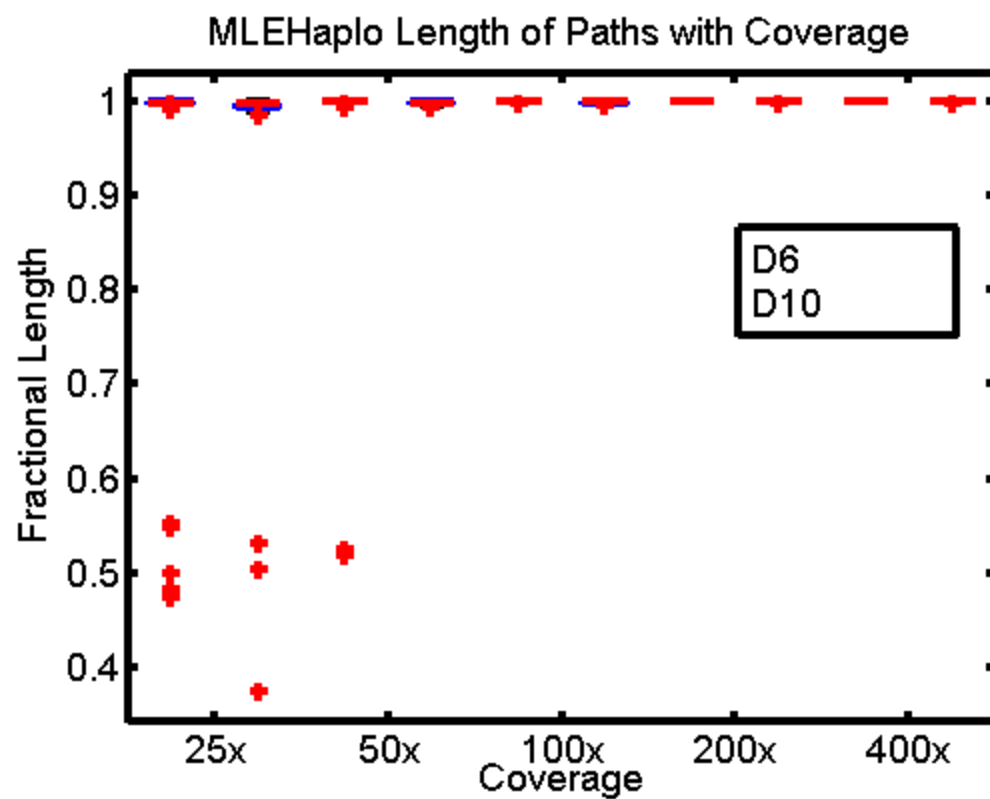

## S5 Figure

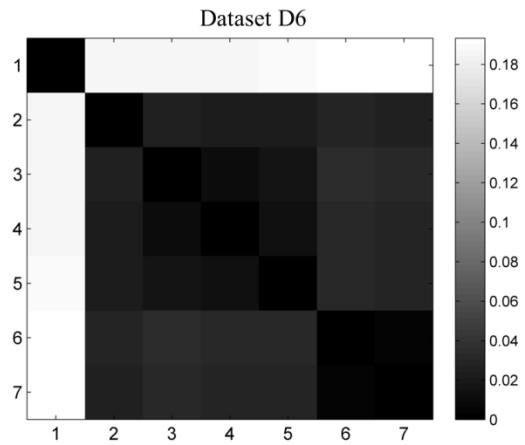

A. D6

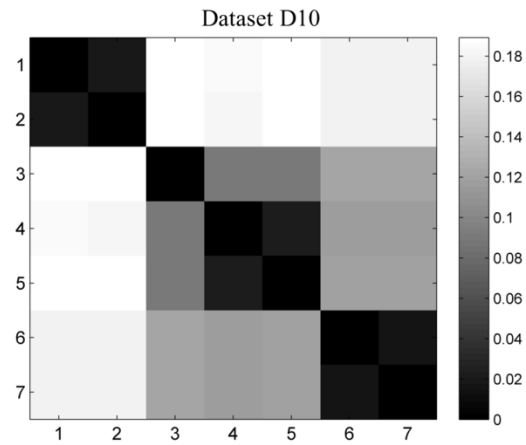

B. D10

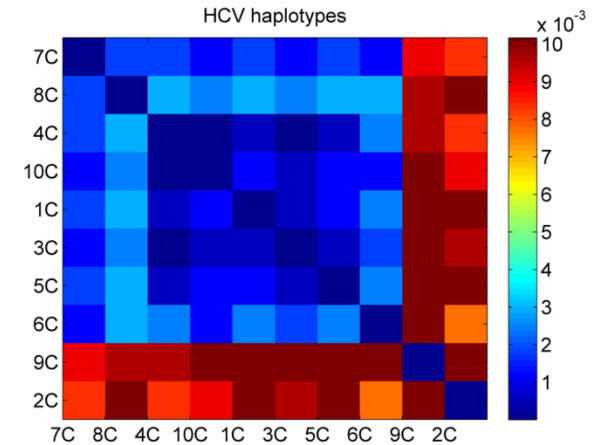

C. HCV haplotypes

## S6 Figure

Distribution of variable sites in the 7 reference sequences for D1

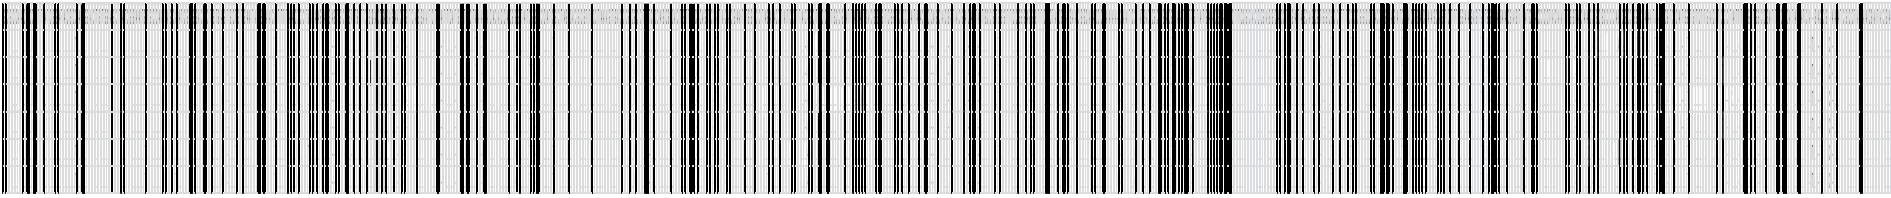

Distribution of variable sites in the E1/E2 genes of 10 HCV Strains

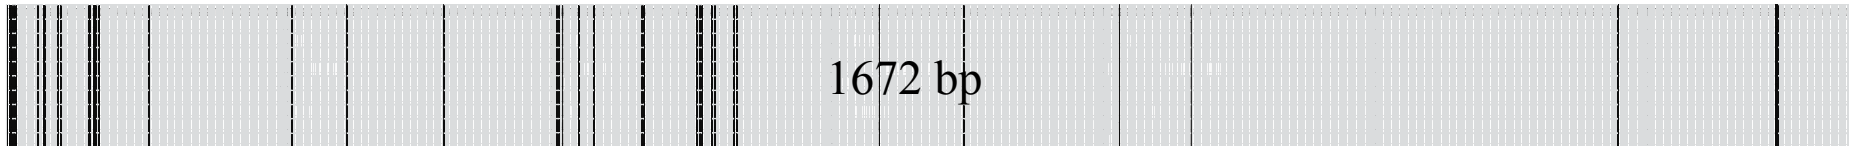

## S7 Figure

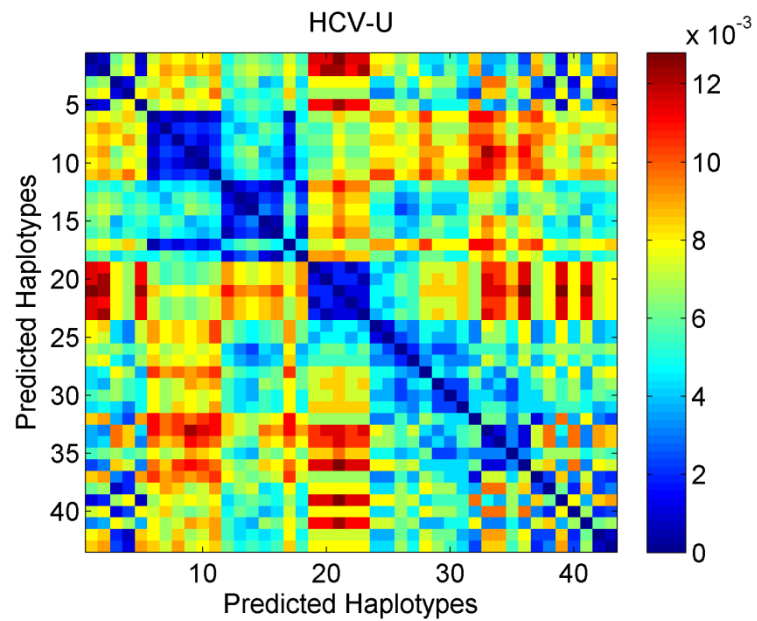

(A)

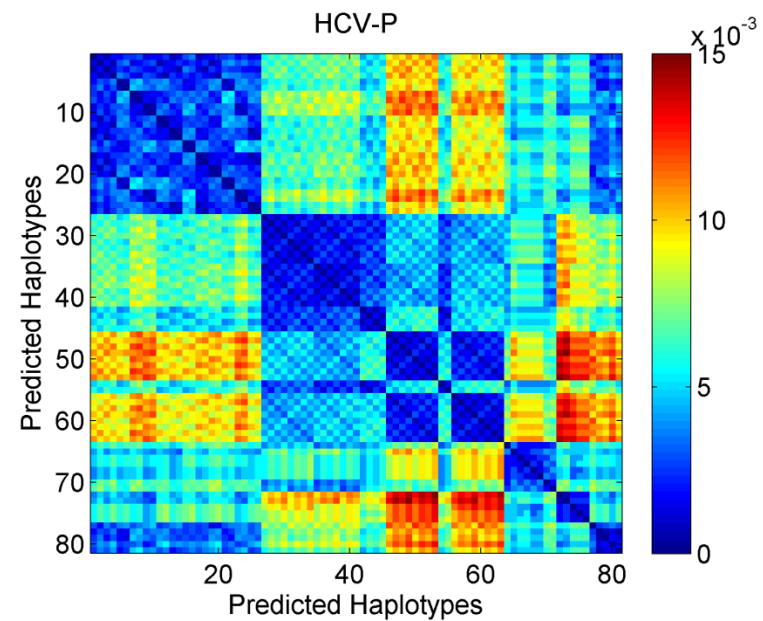

(B)

**S8 Figure**

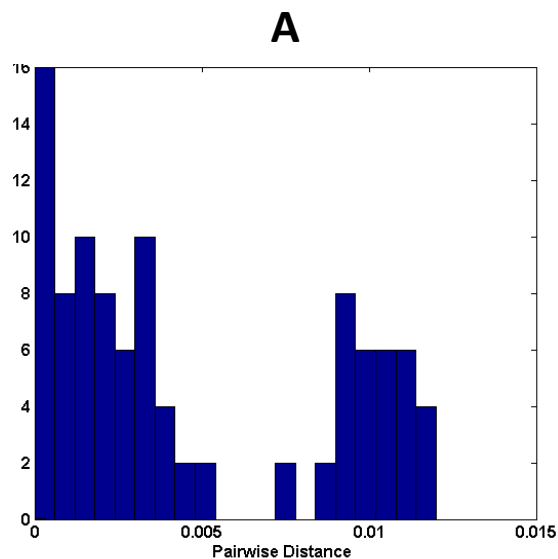

**Ground Truth**

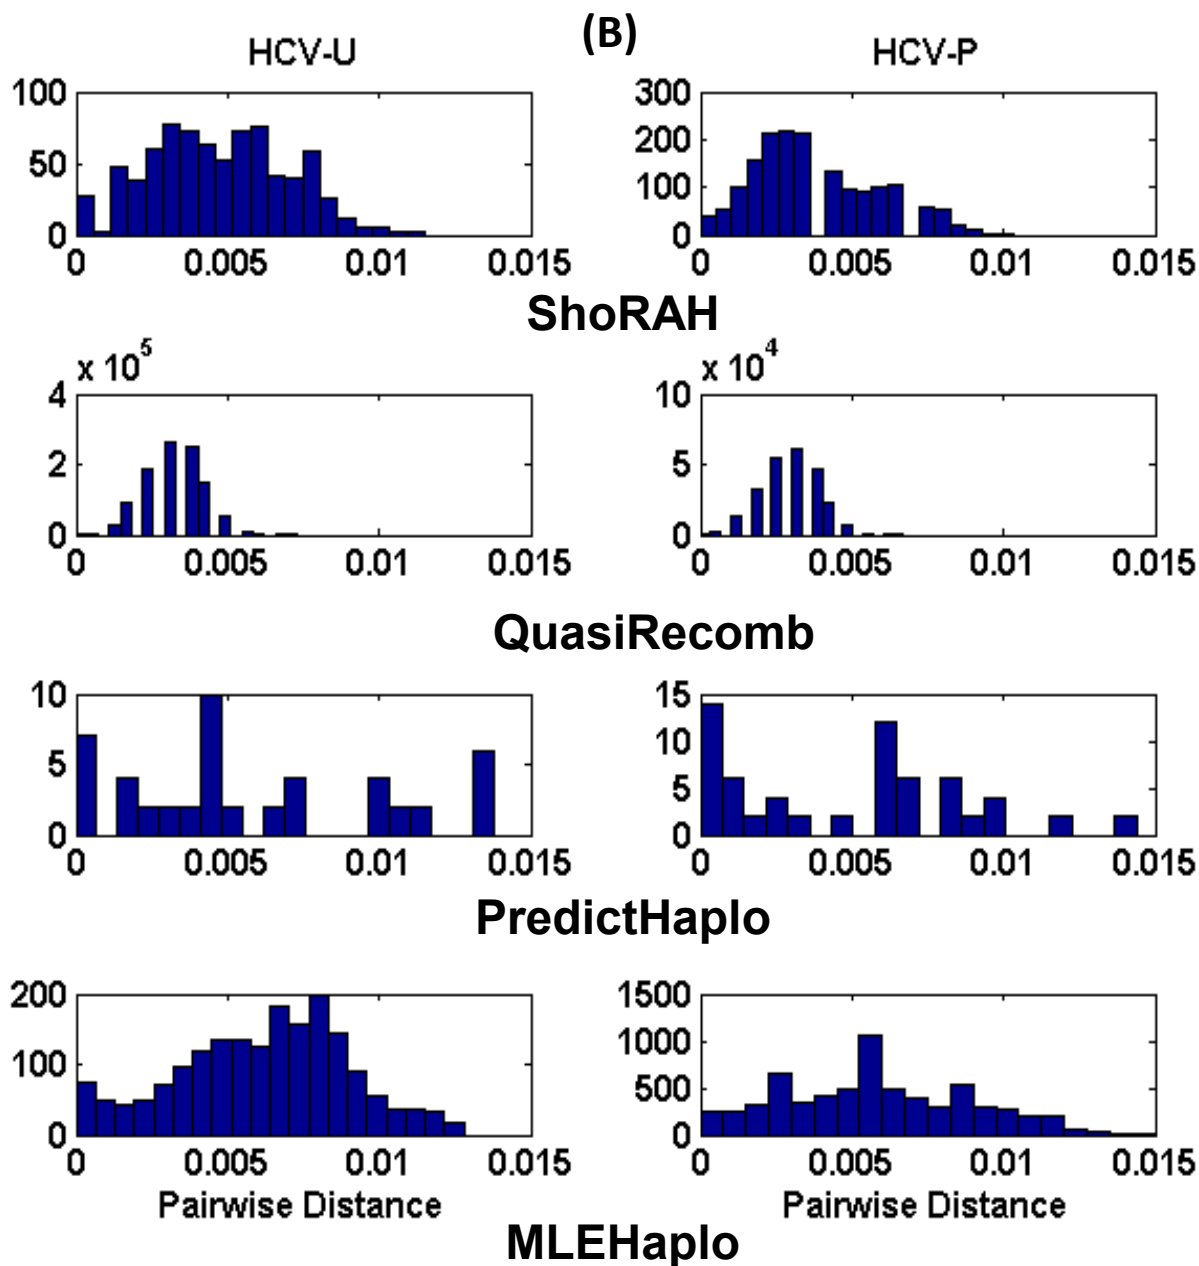



## S9 Figure

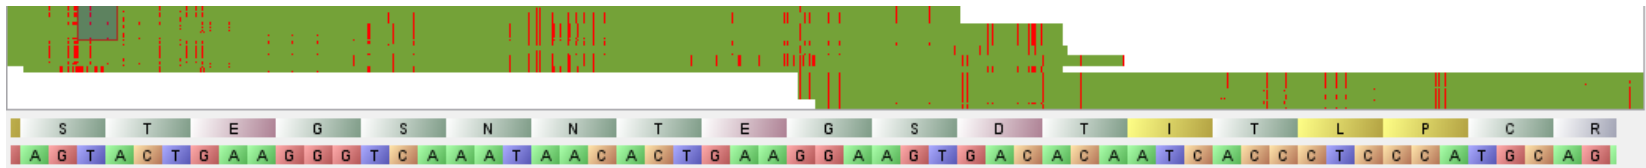

## HXB2

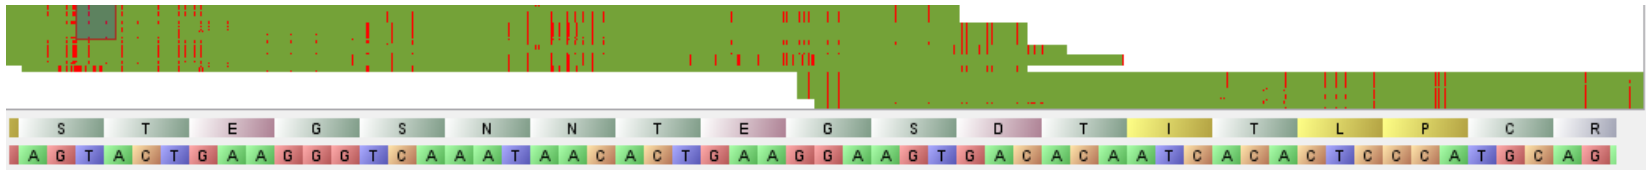

## NL43

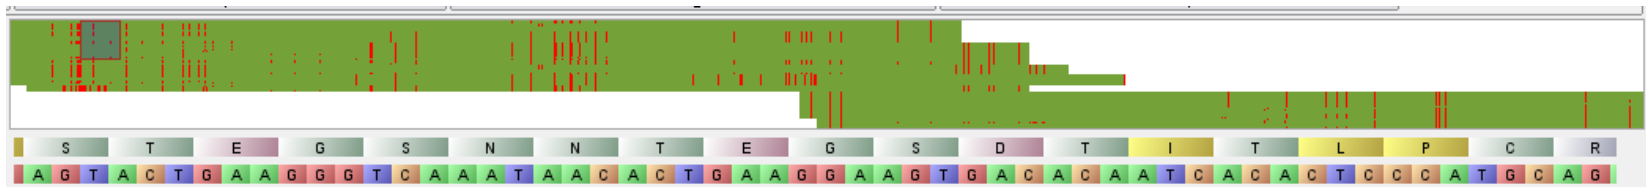

## YU2

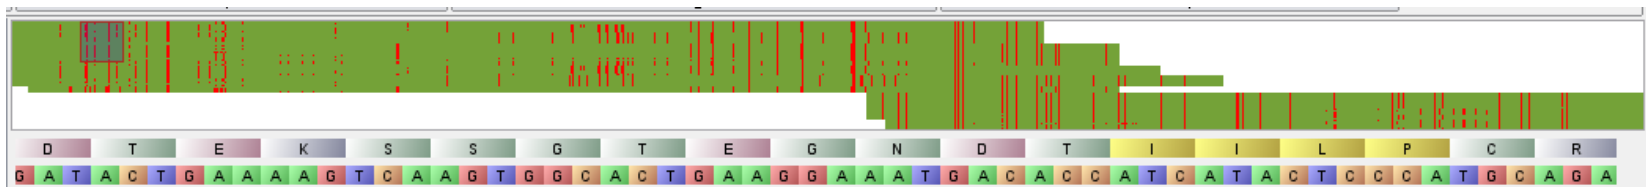

## JRCSF

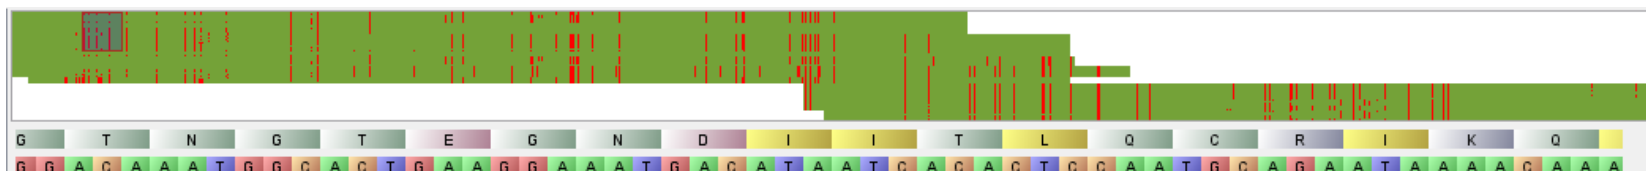

89.6
